# Supplementary material for: Towards Robust and Parameter-Efficient Knowledge Unlearning for LLMs
Source: arXiv:2408.06621 source file (2025-04-24)
Supplement: Supplementary file 1 [file supplementary.tex]

% \documentclass{article}


% % if you need to pass options to natbib, use, e.g.:
% %     \PassOptionsToPackage{numbers, compress}{natbib}
% % before loading neurips_2024


% % ready for submission
% \usepackage{neurips_2024}


% % to compile a preprint version, e.g., for submission to arXiv, add add the
% % [preprint] option:
% %     \usepackage[preprint]{neurips_2024}


% % to compile a camera-ready version, add the [final] option, e.g.:
% %     \usepackage[final]{neurips_2024}


% % to avoid loading the natbib package, add option nonatbib:
% %    \usepackage[nonatbib]{neurips_2024}


% \usepackage[utf8]{inputenc} % allow utf-8 input
% \usepackage[T1]{fontenc}    % use 8-bit T1 fonts
% \usepackage{hyperref}       % hyperlinks
% \usepackage{url}            % simple URL typesetting
% \usepackage{booktabs}       % professional-quality tables
% \usepackage{amsfonts}       % blackboard math symbols
% \usepackage{nicefrac}       % compact symbols for 1/2, etc.
% \usepackage{microtype}      % microtypography
% \usepackage{xcolor}         % colors

% \usepackage{amsmath}
% \usepackage{dsfont}
% \usepackage{graphicx}
% \usepackage{mathtools}
% \usepackage{multirow}
% \usepackage{subcaption}
% \usepackage{wrapfig}

% \input{math_commands}

% \newcommand{\todo}[1]{\textcolor{blue}{TODO: #1}}
% \newcommand\csm[1]{\textcolor{purple}{#1}}


% \title{Towards Parameter-Efficient Unlearning\\ for Large Language Models}


% % The \author macro works with any number of authors. There are two commands
% % used to separate the names and addresses of multiple authors: \And and \AND.
% %
% % Using \And between authors leaves it to LaTeX to determine where to break the
% % lines. Using \AND forces a line break at that point. So, if LaTeX puts 3 of 4
% % authors names on the first line, and the last on the second line, try using
% % \AND instead of \And before the third author name.


% \author{%
%   David S.~Hippocampus\thanks{Use footnote for providing further information
%     about author (webpage, alternative address)---\emph{not} for acknowledging
%     funding agencies.} \\
%   Department of Computer Science\\
%   Cranberry-Lemon University\\
%   Pittsburgh, PA 15213 \\
%   \texttt{hippo@cs.cranberry-lemon.edu} \\
%   % examples of more authors
%   % \And
%   % Coauthor \\
%   % Affiliation \\
%   % Address \\
%   % \texttt{email} \\
%   % \AND
%   % Coauthor \\
%   % Affiliation \\
%   % Address \\
%   % \texttt{email} \\
%   % \And
%   % Coauthor \\
%   % Affiliation \\
%   % Address \\
%   % \texttt{email} \\
%   % \And
%   % Coauthor \\
%   % Affiliation \\
%   % Address \\
%   % \texttt{email} \\
% }


% \begin{document}


% \maketitle


% \begin{abstract}
% Large Language Models (LLMs) have demonstrated strong reasoning and memorization capabilities via pretraining on massive textual corpora. However, training LLMs on human-written text entails significant risk of privacy and copyright infringements, which demands an efficient machine unlearning framework to remove knowledge of sensitive data without retraining the model from scratch. While Gradient Ascent (GA) is widely used to reduce the likelihood of generating unwanted information, the unboundedness of increasing the cross-entropy loss causes not only unstable optimization, but also catastrophic forgetting of knowledge that needs to be retained. We also discover its joint application under low-rank adaptation to be significantly suboptimal in terms of computational cost required for sufficient unlearning as well as post-unlearning generative performance. In response, we propose two novel techniques for effective Low-Rank Unlearning (LoRU). We first design an inverted hinge loss that suppresses unwanted tokens by increasing the probability of the next most likely token, thereby retaining fluency and structure in language generation. We also propose to initialize low-rank adapters based on Fisher information-weighted low-rank approximation, which focuses unlearning on parameters that pertain more to textual data we wish to remove and less to others. Extensive experiments on LM-Eval, Dialogue, and TOFU benchmarks using Neo-GPT, Phi, and Llama2 LLMs show that our approach can efficiently remove unwanted information with negligible deterioration in predictive quality.
% %Large Language Models (LLMs) have demonstrated strong reasoning and memorization capabilities via pretraining on massive textual corpora. However, use of human-written text inevitably leads to privacy and copyright violations of LLMs, which demands an efficient machine unlearning framework that effectively removes knowledge of sensitive data without retraining the LLM from scratch. While gradient ascent provides a simple approach of LLM unlearning by reducing the probability of generating unwanted information, the unbounded nature of increasing the next-token prediction loss not only leads to unstable optimization, but also induces catastrophic forgetting of previously acquired natural language understanding capabilities. In response, we propose projected gradient ascent, a novel LLM unlearning framework that uses non-sensitive data to designate a parameter space that represents knowledge to retain, and finetune the model with gradients projected to its orthogonal space such that unlearning is specified to sensitive information only. To allow stable convergence, we also derive a customized hinge loss that allows straightforward optimization without the need of heuristics for early stopping. Testing our approach on widely used LM benchmarks using Neo-GPT 125M, 1.3B, and 2.7B shows that our approach effectively removes sensitive information with negligible deterioration in predictive quality.
% \end{abstract}


% \input{1_introduction}
% \input{2_related_work}
% \input{3_method}
% \input{4_experiments}
% \input{5_concluding_remarks}

% {\small
% \bibliographystyle{plain}
% \bibliography{reference.bib}
% }
% \newpage

% %%%%%%%%%%%%%%%%%%%%%%%%%%%%%%%%%%%%%%%%%%%%%%%%%%%%%%%%%%%%

% \appendix

% \section{Appendix / supplemental material}


% Optionally include supplemental material (complete proofs, additional experiments and plots) in appendix.
% All such materials \textbf{SHOULD be included in the main submission.}

% %%%%%%%%%%%%%%%%%%%%%%%%%%%%%%%%%%%%%%%%%%%%%%%%%%%%%%%%%%%%

% \end{document}
